# Supplementary material for: Exploring Monotone Priority Queues for Dijkstra Optimization
Source: arXiv:2409.06061 source file (2024-10-16)
Supplement: Supplementary file 1 [file appendix.tex]

\section{Styles of lists, enumerations, and descriptions}\label{sec:itemStyles}

List of different predefined enumeration styles:

\begin{itemize}
\item \verb|\begin{itemize}...\end{itemize}|
\item \dots
\item \dots
%\item \dots
\end{itemize}

\begin{enumerate}
\item \verb|\begin{enumerate}...\end{enumerate}|
\item \dots
\item \dots
%\item \dots
\end{enumerate}

\begin{alphaenumerate}
\item \verb|\begin{alphaenumerate}...\end{alphaenumerate}|
\item \dots
\item \dots
%\item \dots
\end{alphaenumerate}

\begin{romanenumerate}
\item \verb|\begin{romanenumerate}...\end{romanenumerate}|
\item \dots
\item \dots
%\item \dots
\end{romanenumerate}

\begin{bracketenumerate}
\item \verb|\begin{bracketenumerate}...\end{bracketenumerate}|
\item \dots
\item \dots
%\item \dots
\end{bracketenumerate}

\begin{description}
\item[Description 1] \verb|\begin{description} \item[Description 1]  ...\end{description}|
\item[Description 2] Fusce eu leo nisi. Cras eget orci neque, eleifend dapibus felis. Duis et leo dui. Nam vulputate, velit et laoreet porttitor, quam arcu facilisis dui, sed malesuada risus massa sit amet neque.
\item[Description 3]  \dots
%\item \dots
\end{description}

\cref{testenv-proposition} and \autoref{testenv-proposition} ...

\section{Theorem-like environments}\label{sec:theorem-environments}

List of different predefined enumeration styles:

\begin{theorem}\label{testenv-theorem}
Fusce eu leo nisi. Cras eget orci neque, eleifend dapibus felis. Duis et leo dui. Nam vulputate, velit et laoreet porttitor, quam arcu facilisis dui, sed malesuada risus massa sit amet neque.
\end{theorem}

\begin{lemma}\label{testenv-lemma}
Fusce eu leo nisi. Cras eget orci neque, eleifend dapibus felis. Duis et leo dui. Nam vulputate, velit et laoreet porttitor, quam arcu facilisis dui, sed malesuada risus massa sit amet neque.
\end{lemma}

\begin{corollary}\label{testenv-corollary}
Fusce eu leo nisi. Cras eget orci neque, eleifend dapibus felis. Duis et leo dui. Nam vulputate, velit et laoreet porttitor, quam arcu facilisis dui, sed malesuada risus massa sit amet neque.
\end{corollary}

\begin{proposition}\label{testenv-proposition}
Fusce eu leo nisi. Cras eget orci neque, eleifend dapibus felis. Duis et leo dui. Nam vulputate, velit et laoreet porttitor, quam arcu facilisis dui, sed malesuada risus massa sit amet neque.
\end{proposition}

\begin{conjecture}\label{testenv-conjecture}
Fusce eu leo nisi. Cras eget orci neque, eleifend dapibus felis. Duis et leo dui. Nam vulputate, velit et laoreet porttitor, quam arcu facilisis dui, sed malesuada risus massa sit amet neque.
\end{conjecture}

\begin{observation}\label{testenv-observation}
Fusce eu leo nisi. Cras eget orci neque, eleifend dapibus felis. Duis et leo dui. Nam vulputate, velit et laoreet porttitor, quam arcu facilisis dui, sed malesuada risus massa sit amet neque.
\end{observation}

\begin{exercise}\label{testenv-exercise}
Fusce eu leo nisi. Cras eget orci neque, eleifend dapibus felis. Duis et leo dui. Nam vulputate, velit et laoreet porttitor, quam arcu facilisis dui, sed malesuada risus massa sit amet neque.
\end{exercise}

\begin{definition}\label{testenv-definition}
Fusce eu leo nisi. Cras eget orci neque, eleifend dapibus felis. Duis et leo dui. Nam vulputate, velit et laoreet porttitor, quam arcu facilisis dui, sed malesuada risus massa sit amet neque.
\end{definition}

\begin{example}\label{testenv-example}
Fusce eu leo nisi. Cras eget orci neque, eleifend dapibus felis. Duis et leo dui. Nam vulputate, velit et laoreet porttitor, quam arcu facilisis dui, sed malesuada risus massa sit amet neque.
\end{example}

\begin{note}\label{testenv-note}
Fusce eu leo nisi. Cras eget orci neque, eleifend dapibus felis. Duis et leo dui. Nam vulputate, velit et laoreet porttitor, quam arcu facilisis dui, sed malesuada risus massa sit amet neque.
\end{note}

\begin{note*}
Fusce eu leo nisi. Cras eget orci neque, eleifend dapibus felis. Duis et leo dui. Nam vulputate, velit et laoreet porttitor, quam arcu facilisis dui, sed malesuada risus massa sit amet neque.
\end{note*}

\begin{remark}\label{testenv-remark}
Fusce eu leo nisi. Cras eget orci neque, eleifend dapibus felis. Duis et leo dui. Nam vulputate, velit et laoreet porttitor, quam arcu facilisis dui, sed malesuada risus massa sit amet neque.
\end{remark}

\begin{remark*}
Fusce eu leo nisi. Cras eget orci neque, eleifend dapibus felis. Duis et leo dui. Nam vulputate, velit et laoreet porttitor, quam arcu facilisis dui, sed malesuada risus massa sit amet neque.
\end{remark*}

\begin{claim}\label{testenv-claim}
Fusce eu leo nisi. Cras eget orci neque, eleifend dapibus felis. Duis et leo dui. Nam vulputate, velit et laoreet porttitor, quam arcu facilisis dui, sed malesuada risus massa sit amet neque.
\end{claim}

\begin{claim*}\label{testenv-claim2}
Fusce eu leo nisi. Cras eget orci neque, eleifend dapibus felis. Duis et leo dui. Nam vulputate, velit et laoreet porttitor, quam arcu facilisis dui, sed malesuada risus massa sit amet neque.
\end{claim*}

\begin{proof}
Fusce eu leo nisi. Cras eget orci neque, eleifend dapibus felis. Duis et leo dui. Nam vulputate, velit et laoreet porttitor, quam arcu facilisis dui, sed malesuada risus massa sit amet neque.
\end{proof}

\begin{claimproof}
Fusce eu leo nisi. Cras eget orci neque, eleifend dapibus felis. Duis et leo dui. Nam vulputate, velit et laoreet porttitor, quam arcu facilisis dui, sed malesuada risus massa sit amet neque.
\end{claimproof}
